# Supplementary material for: The passive polymer problem
Source: arXiv:chao-dyn/9911005 source file (2000-07-07)
Supplement: Supplementary file 1 [file appendices.tex]

\section{Appendices}

\subsection{Some integrals}
\label{a:Some integrals}
For a $d$-dimensional rotationally invariant integral over $p$, 
which may be $\int_p=\int \rmd^d p\, \rme^{-\sum_{i=1}^d \lambda_i p_i^2}$, we have with some constant $C$
\be
\int_p =\int \rmd^d p\, \rme^{-\sum_{i=1}^d \lambda_i p_i^2}
= C \frac1{\sqrt{\prod_{i=1}^d \lambda_i}}
\ .
\ee
In the case that all $\lambda_i$ equal $\lambda$, the latter
reads with the same constant $C$ 
\be
\int \rmd^d p\, \rme^{- \lambda p^2}
= C \lambda^{-d/2} \ .
\ee
Using this, we obtain by differentiating with respect to 
$\lambda_i$ moments of $p_i$; e.g.
\bea
\left[\int_p p^2\right]^{-1}{\int_p p_1^2}&=& \frac1 d \\
\label{a:2}
\left[{\int_p (p^2)^2}\right]^{-1}{\int_p (p_1)^4}&=& \frac3 {d(d+2)} \\
\label{a:3}
\left[{\int_p (p^2)^2}\right]^{-1}{\int_p p_1^2p_2^2}&=& \frac1 {d(d+2)}
\ .
\eea
Another intelligent way of doing this is to study
\be
\int_p \rme^{- p^2/2} \rme^{ \lambda  p} = C' \rme^{-\lambda^2/2}
\ .
\ee
This yields e.g.
\be
\left[\int_p (p^2)^2\right]^{-1} \int_p (ap)(bp)(cp)(dp)
=\frac1{d(d+2)}\left[ (ab)(cd)+(ac)(bd)+(ad)(bc)\right] \ ,
\ee
where the global prefactor is most easily checked by setting 
$a=b=c=d$ and comparing with \Eq{a:2}. We need
\be
\left[ \int_p (p^2)^2\right]^{-1} \int_p (xp) (yp) (lp)^2
=\frac{1}{d(d+2)}\left( (xy) l^2 +2 (lx)(ly)\right)
\ .
\ee
